# Supplementary material for: OrcVIO: Object residual constrained Visual-Inertial Odometry
Source: arXiv:2007.15107 source file (2021-05-29)
Supplement: Supplementary file 1 [file Additional.tex]

\section{Additional Derivations}
\label{sec:additional}

\subsection{Alternative Bounding-box Residual Formulation}
\label{sec:alternative-bbox-residual-explanation}

If the dual ellipsoid $\bfQ_{(\bfu+\delta\bfu)}^*$ of instance $\bfo_i$ is estimated accurately, then the lines ${}^{b}_{}\underline{\mathbf{z}}_{t,j,k}$ of the $k$-th bounding-box at time $t$ should be tangent to the image plane conic projection of $\bfQ_{(\bfu+\delta\bfu)}^*$, then we could define the residual in this way:
\begin{equation}
\label{eq:bb-error}
\scaleMathLine[0.89]{{}^b\bfe(\bfx, \bfo, {}^b\underline{\mathbf{z}}) \triangleq {}^b\underline{\mathbf{z}}^\top \bfP {}_C\bfT^{-1}\! {}_O\bfT \bfQ_{(\bfu+\delta\bfu)}^*  {}_O\bfT^\top  {}_C\bfT^{-\!\top} \bfP^\top {}^b\underline{\mathbf{z}}.}
\end{equation}

% \SHAN{need to change to correct perturbation}
The Jacobians of ${}^b\bfe$ with respect to perturbations ${}_{C}\bfxi_t, {}_{O}\bfxi, \delta\tilde{\bfu}$, evaluated at estimates $\hat{\bfx}_t$, $\hat{\bfo}$, are:
\begin{align}
\frac{\partial{}^b\bfe}{\partial{}_{C}\bfxi_t} &= -2 {}^b\underline{\mathbf{z}}^\top \bfP {}_C\hat{\bfT}_t^{-1} {}_O\hat{\bfT} \hat{\bfQ}_{(\bfu+\delta\hat{\bfu})}^* {}_O\hat{\bfT}^\top {}_C\hat{\bfT}_t^{-\top} 
\brl{\bfP^\top {}^b\underline{\mathbf{z}}}^{\circledcirc \top}\notag\\
\frac{\partial{}^b\bfe}{\partial{}_{O}\bfxi} &= 2 {}^b\underline{\mathbf{z}}^\top \bfP {}_C\hat{\bfT}_t^{-1} {}_O\hat{\bfT} \hat{\bfQ}_{(\bfu+\delta\hat{\bfu})}^* 
\brl{{}_O\hat{\bfT}^\top {}_C\hat{\bfT}_t^{-\top} \bfP^\top {}^b\underline{\mathbf{z}}}^{\circledcirc \top}\notag\\
\frac{\partial{}^b\bfe}{\partial\delta\tilde{\bfu}} &= (2 (\bfu+\delta\hat{\bfu}) \odot \bfy \odot \bfy)^\top \in \mathbb{R}^{1 \times 3}\\
\bfy & \triangleq \begin{bmatrix} \bfI_{3} & \mathbf{0} \end{bmatrix} {}_O\hat{\bfT}^\top  {}_C\hat{\bfT}_t^{-\top} \bfP^\top {}^b\underline{\mathbf{z}}\notag
\end{align}
where $\odot$ denotes element wise multiplication.
The Jacobians with resp. to other perturbations in~\eqref{eq:perturbations} are $\mathbf{0}$. 
Hence, $\frac{\partial {}^b\hat{\bfe}}{\partial \tilde{\bfo}} = \brl{\frac{\partial{}^b\bfe}{\partial{}_{O}\bfxi}\ \frac{\partial{}^b\bfe}{\partial\delta\tilde{\bfu}}\ \bf0} \in \mathbb{R}^{1 \times \prl{6 + 3 + 3N_s}}$, which is used in \eqref{eq:object-lm}. 

The proofs are as follows. Starting from \eqref{eq:bb-error}, let 
\begin{equation} 
\begin{aligned}
a \triangleq {}^b\underline{\mathbf{z}}^\top \bfP {}_C\bfT^{-1}\! {}_O\bfT \bfQ_{(\bfu+\delta\bfu)}^*  {}_O\bfT^\top  {}_C\bfT^{-\!\top} \bfP^\top {}^b\underline{\mathbf{z}}
\\
\bfb \triangleq {}_O\bfT^\top  {}_C\bfT^{-\!\top} \bfP^\top {}^b\underline{\mathbf{z}}
\quad 
a = \bfb^\top \bfQ_{(\bfu+\delta\bfu)}^* \bfb. 
\end{aligned}
\end{equation}
Therefore
% \begin{equation}
% % \label{eq:bb-jacobians-proof1a}
% \begin{aligned}
% \frac{\partial{}^b\bfe}{\partial{}_{C}\bfxi_t} 
% =
% \frac{d a}{d \bfb} \frac{d \bfb}{d {}_{C}\bfxi_t}
% \end{aligned}
% \end{equation}
$
\frac{\partial{}^b\bfe}{\partial{}_{C}\bfxi_t} 
=
\frac{d a}{d \bfb} \frac{d \bfb}{d {}_{C}\bfxi_t}
$,
where 
\begin{equation}
% \label{eq:bb-jacobians-proof1b}
\begin{aligned}
\frac{d a}{d \bfb} 
&= 
\bfb^\top \prl{\bfQ_{(\bfu+\delta\bfu)}^* + \bfQ_{(\bfu+\delta\bfu)}^{*\top}}\\
&=
{}^b\underline{\mathbf{z}}^\top \bfP {}_C\bfT^{-1}\! {}_O\bfT \prl{\bfQ_{(\bfu+\delta\bfu)}^* + \bfQ_{(\bfu+\delta\bfu)}^{*\top}} \\ 
&= 
2 {}^b\underline{\mathbf{z}}^\top \bfP {}_C\bfT^{-1}\! {}_O\bfT \bfQ_{(\bfu+\delta\bfu)}^*, 
\end{aligned}
\end{equation}
for which we use 
% \begin{equation}
% \frac{\partial \mathbf{x}^{\top} \mathbf{B} \mathbf{x}}{\partial \mathbf{x}}= \mathbf{x}^\top \left(\mathbf{B}+\mathbf{B}^{\top}\right) 
% \end{equation}
$
\frac{\partial \mathbf{x}^{\top} \mathbf{B} \mathbf{x}}{\partial \mathbf{x}}= \mathbf{x}^\top \left(\mathbf{B}+\mathbf{B}^{\top}\right) 
$.

For the third equation
% \begin{equation}
% % \label{eq:bb-jacobians-proof3}
% \begin{aligned}
% \frac{\partial {}^b\bfe(\bfx, \bfo, {}^b\underline{\mathbf{z}})}{\partial \delta\tilde{\bfu}_i} 
% &=
% \bfy^\top \text{diag}\prl{2 (\bfu+\delta\hat{\bfu})} \bfy \\
% &=
% (2 (\bfu+\delta\hat{\bfu}) \odot \bfy \odot \bfy)^\top
% \end{aligned}
% \end{equation}
\begin{equation}
\begin{aligned}
\scaleMathLine[0.95]{
\frac{\partial {}^b\bfe(\bfx, \bfo, {}^b\underline{\mathbf{z}})}{\partial \delta\tilde{\bfu}_i} 
=
\bfy^\top \text{diag}\prl{2 (\bfu+\delta\hat{\bfu})} \bfy 
=
(2 (\bfu+\delta\hat{\bfu}) \odot \bfy \odot \bfy)^\top
}. 
\end{aligned}
\end{equation}

However, the magnitude of this residual is quadratic with respect to $\bfb$, which will make the optimization of the cost function more difficult for two reasons: the relative pose of the object in the camera frame could be large, and the magnitude of the residual is much higher than the reprojection error. To tackle these issues we have to carefully tune the weights in the object LM, which could make the system brittle.  
Thus, we propose another form of the residual used in the main paper that is in the same units as the reprojection error.

\subsection{Full Proof of IMU Propagation}
\label{sec:imu-integral-proof}

To prove \eqref{eq:imu-integral}, starting from \eqref{eq:imu-error-dynamics-nominal}, 
for the first row,
% \begin{align}
% {}_I\hat{\bfR}(t+\tau)
% &=
% {}_I\hat{\bfR}_{t} 
% \exp\left(\int_{t}^{t+\tau} \bigl({}^i\bfomega_t \!- \hat{\bfb}_{g,t}\bigr)_{\times} ds\right)\notag\\
% &=
% {}_I\hat{\bfR}_{t}
% \exp\prl{\tau \bigl({}^i\bfomega_t \!- \hat{\bfb}_{g,t}\bigr)_{\times}}
% \end{align}
% \begin{align*}
% {}_I\hat{\bfR}(t+\tau)
% =
% {}_I\hat{\bfR}_{t}
% \exp\prl{\tau \bigl({}^i\bfomega_t \!- \hat{\bfb}_{g,t}\bigr)_{\times}}
% \end{align*}
\begin{equation}
\begin{aligned}
{}_I\hat{\bfR}_{t+1}^{p} =  {}_I\hat{\bfR}(t+\tau) = 
{}_I\hat{\bfR}_{t}
\exp\prl{\tau \bigl({}^i\bfomega_t \!- \hat{\bfb}_{g,t}\bigr)_{\times}}. 
\end{aligned}
\end{equation}

% \begin{align}
% {}_I\hat{\bfR}_{t+1}^{p} =  {}_I\hat{\bfR}(t+\tau) = 
% {}_I\hat{\bfR}_{t}
% \exp\prl{\tau \bigl({}^i\bfomega_t \!- \hat{\bfb}_{g,t}\bigr)_{\times}}
% \end{align}

For the fourth row, 
\begin{equation}
\begin{aligned}
\label{eq:imu_integral_v}
&{}_I\hat{\bfv}_{t+1}^{p}
=
{}_I\hat{\bfv}_{t} 
+
\int_{t}^{t+\tau} {}_I\dot{\hat{\bfv}}_{t} ds\\
&=
{}_I\hat{\bfv}_{t} 
+
\int_{t}^{t+\tau} {}_I\hat{\bfR}(s) \prl{{}^i\bfa - \hat{\bfb}_a} ds +
\int_{t}^{t+\tau} \bfg ds \\
&= 
{}_I\hat{\bfv}_{t} + \bfg \tau +
\int_{t}^{t+\tau} {}_I\hat{\bfR}(s) \prl{{}^i\bfa - \hat{\bfb}_a} ds \\
&=
{}_I\hat{\bfv}_{t} + \bfg \tau +
\int_{t}^{t+\tau} {}_I\hat{\bfR}(s) ds \prl{{}^i\bfa - \hat{\bfb}_a}  \\
&= 
{}_I\hat{\bfv}_{t} + \bfg \tau + {}_I\hat{\bfR}_t \int_{0}^{\tau} \exp\prl{s \bigl({}^i\bfomega_t \!- \hat{\bfb}_{g,t}\bigr)_{\times}} ds \prl{{}^i\bfa - \hat{\bfb}_a}. 
\end{aligned}
\end{equation}
The integral in the last term in the right hand side of \eqref{eq:imu_integral_v} could be expressed as
\begin{equation} 
\begin{aligned}
&\int_{0}^{\tau} \exp\prl{s \bigl({}^i\bfomega_t \!- \hat{\bfb}_{g,t}\bigr)_{\times}} ds  \\
&= 
\int_{0}^{\tau} \sum_{n=0}^{\infty} \frac{1}{n !} \prl{s \bigl({}^i\bfomega_t \!- \hat{\bfb}_{g,t}\bigr)_{\times}}^n ds  \\ 
&= 
\sum_{n=0}^{\infty} \frac{1}{n !} \int_{0}^{\tau} \prl{s \bigl({}^i\bfomega_t \!- \hat{\bfb}_{g,t}\bigr)_{\times}}^n ds  \\
&=
\sum_{n=0}^{\infty} \frac{1}{\prl{n+1} !} \tau^{n+1} \prl{ \bigl({}^i\bfomega_t \!- \hat{\bfb}_{g,t}\bigr)_{\times}}^n  \\
&= 
\tau \sum_{n=0}^{\infty} \frac{1}{\prl{n+1} !} \prl{\tau \bigl({}^i\bfomega_t \!- \hat{\bfb}_{g,t}\bigr)_{\times}}^n. 
\end{aligned}
\end{equation}
Hence we are left to show that 
\begin{equation}
\label{eq:J_l}
\begin{aligned}
\scaleMathLine[0.8]{
\sum_{n=0}^{\infty} \frac{1}{\prl{n+1} !} \prl{\tau \bigl({}^i\bfomega_t \!- \hat{\bfb}_{g,t}\bigr)_{\times}}^n
= 
\bfJ_L\!\prl{\tau \bigl({}^i\bfomega_t \!- \hat{\bfb}_{g,t}\bigr)}
}. 
\end{aligned}
\end{equation}
Let $\boldsymbol\omega = \tau \bigl({}^i\bfomega_t \!- \hat{\bfb}_{g,t}\bigr)$, and $\bfomega = \phi\bfa$, where $\phi = \|\bfomega\|$, $\bfa = \bfomega/\phi$, then the right hand side of \eqref{eq:J_l} becomes 
% \begin{align}
% &\sum_{n=0}^{\infty} \frac{1}{\prl{n+1} !} \prl{\phi\bfa_{\times}}^n
% = 
% \bfI_3 + \frac{\phi \bfa_\times}{2!} + \frac{\phi^2 \bfa_\times^2}{3!} + \frac{\phi^3 \bfa_\times^3}{4!} + ...
% \notag \\ 
% &=
% % \bfI + \frac{\phi}{2!}\bfa_\times + \frac{\phi^2}{3!}\bfa_\times^2 + \frac{\phi^3}{4!}\prl{-\bfa_\times} + \frac{\phi^4}{5!}\prl{-\bfa_\times \bfa_\times} + \frac{\phi^5}{6!}\bfa_\times + \frac{\phi^6}{7!}\bfa_\times\bfa_\times + ... 
% \bfI_3 + \frac{\phi}{2!}\bfa_\times + \frac{\phi^2}{3!}\bfa_\times^2 + \frac{\phi^3}{4!}\prl{-\bfa_\times} + \frac{\phi^4}{5!}\prl{-\bfa_\times \bfa_\times} + \frac{\phi^5}{6!}\bfa_\times + ... \notag \\ 
% &= 
% \bfI_3 + \prl{\frac{\phi}{2!} - \frac{\phi^3}{4!} + \frac{\phi^5}{6!} - ...}\bfa_\times + \prl{\frac{\phi^2}{3!} - \frac{\phi^4}{5!} + \frac{\phi^6}{7!} - ...}\bfa_\times \bfa_\times \notag \\ 
% \end{align}
\begin{equation}
\begin{aligned}
\scaleMathLine[0.9]{
\bfI_3 + \prl{\frac{\phi}{2!} - \frac{\phi^3}{4!} + \frac{\phi^5}{6!} - ...}\bfa_\times + \prl{\frac{\phi^2}{3!} - \frac{\phi^4}{5!} + \frac{\phi^6}{7!} - ...}\bfa_\times \bfa_\times 
}, 
\end{aligned}
\end{equation}
where we use the property $\bfa_\times \bfa_\times \bfa_\times = -\bfa_\times$ based on (42) in \cite{quatekf}. Using the series expansions of trigonometric functions 
\begin{equation}
\begin{aligned}
\label{eq:tri_series}
\cos \phi
&=
1-\frac{\phi^{2}}{2 !}+\frac{\phi^{4}}{4 !}-\frac{\phi^{6}}{6 !}+\frac{\phi^{8}}{8 !}-\dots \\ 
\sin \phi
&=
\phi-\frac{\phi^{3}}{3 !}+\frac{\phi^{5}}{5 !}-\frac{\phi^{7}}{7 !}+\frac{\phi^{9}}{9 !}-\dots,  
\end{aligned}
\end{equation}
which lead to 
% \begin{align}
% \frac{\phi}{2!} - \frac{\phi^3}{4!} + \frac{\phi^5}{6!} - \dots 
% &= 
% \frac{1}{\phi} \prl{\frac{\phi^2}{2!} - \frac{\phi^4}{4!} + \frac{\phi^6}{6!} - ...} \notag \\ 
% &= 
% \frac{1}{\phi} \prl{1 - \cos \phi}
% \end{align}
% \begin{align}
% \frac{\phi^2}{3!} - \frac{\phi^4}{5!} + \frac{\phi^6}{7!} - \dots 
% &= 
% \frac{1}{\phi} \prl{\frac{\phi^3}{3!} - \frac{\phi^5}{5!} + \frac{\phi^7}{7!} - \dots} \notag \\ 
% &= 
% \frac{1}{\phi} \prl{\phi - \sin \phi}
% \end{align}
\begin{equation}
\begin{aligned}
\frac{\phi}{2!} - \frac{\phi^3}{4!} + \frac{\phi^5}{6!} - \dots 
&= 
\frac{1}{\phi} \prl{1 - \cos \phi}  
\\
\frac{\phi^2}{3!} - \frac{\phi^4}{5!} + \frac{\phi^6}{7!} - \dots 
&= 
\frac{1}{\phi} \prl{\phi - \sin \phi}. 
\end{aligned}
\end{equation}
We also have $\bfa_\times = \frac{\bfomega_\times}{\phi}$, 
% \begin{align}
% \bfa_\times = \frac{\bfomega_\times}{\phi}
% \end{align}
therefore 
% \begin{align}
% &\sum_{n=0}^{\infty} \frac{\bfomega_\times^n}{\prl{n+1} !}
% = \notag \\ 
% &\bfI_3 + \frac{1-\cos\|\bfomega\|}{\|\bfomega\|^2}\bfomega_{\times} + \frac{\|\bfomega\|-\sin\|\bfomega\|}{\|\bfomega\|^3}\bfomega_{\times}^2
% \end{align}
\begin{equation}
\begin{aligned}
\scaleMathLine[1]{
\sum_{n=0}^{\infty} \frac{\bfomega_\times^n}{\prl{n+1} !}
= 
\bfI_3 + \frac{1-\cos\|\bfomega\|}{\|\bfomega\|^2}\bfomega_{\times} + \frac{\|\bfomega\|-\sin\|\bfomega\|}{\|\bfomega\|^3}\bfomega_{\times}^2
}. 
\end{aligned}
\end{equation}

For the third row:
% \begin{align}
% \label{eq:imu_integral_p}
% {}_I\hat{\bfp}_{t+1}^{p}
% &=
% {}_I\hat{\bfp}_{t} 
% +
% \int_{t}^{t+\tau} {}_I\dot{\hat{\bfp}}_{t} ds \notag \\
% &=
% {}_I\hat{\bfp}_{t} 
% +
% \int_{0}^{\tau} {}_I\hat{\bfv}_t + \bfg s + \notag \\
% & {}_I\hat{\bfR}_{t} \bfJ_L\!\prl{s \bigl({}^i\bfomega_t \!- \hat{\bfb}_{g,t}\bigr)} \bigl({}^i\bfa_t \!- \hat{\bfb}_{a,t}\bigr) s ds 
% %  \\ 
% % &= 
% % {}_I\hat{\bfp}_{t} + {}_I\hat{\bfv}_t\tau + \bfg\frac{\tau^2}{2} +
% % {}_I\hat{\bfR}_{t} \int_{t}^{t+\tau} \bfJ_L\!\prl{s \bigl({}^i\bfomega_t \!- \hat{\bfb}_{g,t}\bigr)} ds \bigl({}^i\bfa_t \!- \hat{\bfb}_{a,t}\bigr) \frac{1}{2}\tau^2 
% \end{align}
\begin{equation}
\begin{aligned}
\scaleMathLine[0.95]{
{}_I\hat{\bfp}_{t+1}^{p}
=
{}_I\hat{\bfp}_{t} 
+
\int_{0}^{\tau} {}_I\hat{\bfv}_t + \bfg s + {}_I\hat{\bfR}_{t} \bfJ_L\!\prl{s \bigl({}^i\bfomega_t \!- \hat{\bfb}_{g,t}\bigr)} \bigl({}^i\bfa_t \!- \hat{\bfb}_{a,t}\bigr) s ds
}. 
\end{aligned}
\end{equation}
We are left to show 
\begin{equation}
\label{eq:Jl_to_Hl}
\begin{aligned}
\scaleMathLine[0.8]{
\int_{0}^{\tau} \bfJ_L\!\prl{s \bigl({}^i\bfomega_t \!- \hat{\bfb}_{g,t}\bigr)} s ds 
= 
\tau^2 \bfH_L\!\prl{\tau \bigl({}^i\bfomega_t \!-\!\hat{\bfb}_{g,t}\bigr)}
}. 
\end{aligned}
\end{equation}
Let $\bfomega^\prime = \bigl({}^i\bfomega_t \!- \hat{\bfb}_{g,t}\bigr)$, \eqref{eq:Jl_to_Hl} could be proved as  
\begin{equation}
\begin{aligned}
&\int_{0}^{\tau} \bfJ_L\!\prl{s \bigl({}^i\bfomega_t \!- \hat{\bfb}_{g,t}\bigr)} s ds \\
&= \int_{0}^{\tau} \prl{\bfI_3 + \frac{s\bfomega^\prime_{\times}}{2!} + \frac{(s\bfomega^{\prime2}_{\times})}{3!} + \ldots} s ds \\
&= \int_{0}^{\tau} \prl{s\bfI_3 + \frac{s^2\bfomega^\prime_{\times}}{2!} + \frac{s^3\bfomega^{\prime2}_{\times}}{3!} + \ldots} ds \\
&= \frac{\tau^2}{2}\bfI_3 + \frac{\tau^3\bfomega^\prime_{\times}}{3 \times 2!} + \frac{\tau^4\bfomega^{\prime2}_{\times}}{4 \times 3!} + \ldots \\
&= \tau^2\prl{\frac{\bfI_3}{2} + \frac{\tau\bfomega^\prime_{\times}}{3! } + \frac{\tau^2\bfomega^{\prime2}_{\times}}{4!} + \ldots} \\
&= \tau^2 \bfH_L\!\prl{\tau \bigl({}^i\bfomega_t \!-\!\hat{\bfb}_{g,t}\bigr)}. 
\end{aligned}
\end{equation}

Next we derive the closed-form expression of $\bfH_L$ as follows, let $\boldsymbol\omega = \tau \bigl({}^i\bfomega_t \!- \hat{\bfb}_{g,t}\bigr)$, $\bfomega = \phi\bfa$ as before:
% \begin{align*}
% &\frac{\bfI_3}{2!} + \frac{\bfomega_{\times}}{3!} + \frac{\bfomega_{\times}^2}{4!} + \ldots \notag \\ 
% &= 
% \frac{\bfI_3}{2} + \frac{\phi \bfa_\times}{3!} + \frac{\prl{\phi\bfa_\times}^2}{4!} + \frac{\prl{\phi\bfa_\times}^3}{5!} + 
% \frac{\prl{\phi\bfa_\times}^4}{6!} + \dots \notag \\
% &= 
% \frac{\bfI_3}{2} + \frac{\phi \bfa_\times}{3!} + \frac{\prl{\phi\bfa_\times}^2}{4!} -
% \frac{\prl{\phi}^3}{5!}\bfa_\times - 
% \frac{\prl{\phi}^4}{6!}\bfa_\times^2 + \dots \notag \\
% &= 
% \frac{\bfI_3}{2} +
% \prl{\frac{\phi}{3!} - \frac{\phi^3}{5!} + \dots}\bfa_\times +
% \prl{\frac{\phi^2}{4!} - \frac{\phi^4}{6!} + \dots}\bfa^2_\times
% \end{align*}
\begin{equation}
\begin{aligned}
\scaleMathLine[0.95]{
\frac{\bfI_3}{2!} + \frac{\bfomega_{\times}}{3!} + \frac{\bfomega_{\times}^2}{4!} + \ldots 
= 
\frac{\bfI_3}{2} +
\prl{\frac{\phi}{3!} - \frac{\phi^3}{5!} + \dots}\bfa_\times +
\prl{\frac{\phi^2}{4!} - \frac{\phi^4}{6!} + \dots}\bfa^2_\times
}. 
\end{aligned}
\end{equation}
Furthermore, using the series expansion of trigonometric functions \eqref{eq:tri_series}, we have:
% \begin{align}
% &\frac{\phi}{3!} - \frac{\phi^3}{5!} + \frac{\phi^5}{7!} - \dots \notag \\
% &= 
% \frac{1}{\phi^2} \prl{\frac{\phi^3}{3!} - \frac{\phi^5}{5!} + \frac{\phi^7}{7!} - \dots} \notag \\ 
% &= 
% \frac{1}{\phi^2} \prl{\phi - \sin \phi}
% \end{align}
$
\frac{\phi}{3!} - \frac{\phi^3}{5!} + \frac{\phi^5}{7!} - \dots 
=
\frac{1}{\phi^2} \prl{\phi - \sin \phi}
$.
Hence 
\begin{align}
\prl{\frac{\phi}{3!} - \frac{\phi^3}{5!} + \frac{\phi^5}{7!} - \dots} \bfa_\times = \frac{1}{\phi^3} \prl{\phi - \sin \phi} \bfomega_\times. 
\end{align}
Furthermore, 
\begin{align}
&\frac{\phi^2}{4!} - \frac{\phi^4}{6!} + \frac{\phi^6}{8!} - \dots \notag \\
&= 
\frac{1}{\phi^2}\prl{\frac{\phi^4}{4!} - \frac{\phi^6}{6!} + \frac{\phi^8}{8!} - \dots} \notag \\
&= 
\frac{1}{\phi^2}\prl{-\frac{\phi^2}{2!} + \frac{\phi^4}{4!} - \frac{\phi^6}{6!} + \frac{\phi^8}{8!} - \dots + \frac{\phi^2}{2!}} \notag \\
&= 
\frac{1}{2\phi^2} \prl{2\prl{\cos \phi - 1} + \phi^2}, 
\end{align}
and finally we get 
\begin{equation}
\begin{aligned}
\prl{\frac{\phi^2}{4!} - \frac{\phi^4}{6!} + \frac{\phi^6}{8!} - \dots} \bfa^2_\times = \frac{1}{2\phi^4} \prl{2\prl{\cos \phi - 1} + \phi^2} \bfomega^2_\times. 
\end{aligned}
\end{equation}
Therefore,  
% \begin{multline}
% \bfH_L\prl{\bfomega} = \frac{1}{2}\bfI_3 + \frac{\|\bfomega\|-\sin\|\bfomega\|}{\|\bfomega\|^3}\bfomega_{\times} 
% \\
% + \frac{2(\cos\|\bfomega\|-1)+\|\bfomega\|^2}{2\|\bfomega\|^4}\bfomega_{\times}^2
% \end{multline}
\begin{equation}
\begin{aligned}
\scaleMathLine[0.9]{
\bfH_L\prl{\bfomega} = \frac{1}{2}\bfI_3 + \frac{\|\bfomega\|-\sin\|\bfomega\|}{\|\bfomega\|^3}\bfomega_{\times} 
+ \frac{2(\cos\|\bfomega\|-1)+\|\bfomega\|^2}{2\|\bfomega\|^4}\bfomega_{\times}^2
}. 
\end{aligned}
\end{equation}

\subsection{Comparison of Perturbation Schemes on EuRoC Dataset}
\label{sec:eval_perturbation}

% table for euroc dataset 

\begin{table*}[!tbp]
    \centering
   \caption {RMSE of ATE (deg/meters) on EuRoC} 
   \resizebox{\textwidth}{!}{%
      \begin{tabular}{l rrrrrrrrrrrr}
      \toprule
  EuRoC Sequence $\rightarrow$  & MH 01 & MH 02 & MH 03 & MH 04 & MH 05 & V1 01  & V1 02 & V1 03 & V2 01 & V2 02 & V2 03 & Mean \\ \midrule
  Right perturbation & 1.51/0.11 & \bf{1.58/0.45} & 2.03/0.26 & \bf{1.12/0.34} & 1.38/0.43 &  \bf{1.00/0.12} & 1.64/0.25 & \bf{1.22/0.24} & 0.79/0.09 & 1.18/0.14 & \bf{1.43/0.22} & \bf{1.35/0.24} \\ 
  Left perturbation & \bf{1.50/0.10} & 2.14/0.57 & \bf{1.50/0.42} & 2.38/0.40 & \bf{1.14/0.37} & 1.06/0.12 & 2.16/0.14 & 2.41/0.25 & 0.63/0.11 & \bf{1.14/0.14} & 1.60/0.22 & 1.60/0.26 \\
  \bottomrule
    \end{tabular}
    }
  \label{tab:eval_perturb_euroc}
  \end{table*}

To evaluate the performance of left perturbation with respect to the right perturbation, the ATE in degrees and meters on the EuRoC dataset \cite{burri2016euroc} are show in Table \ref{tab:eval_perturb_euroc}. It could be observed from the table that right perturbation leads to better accuracy than the left perturbation.
